# Supplementary material for: Laplacian Constrained Precision Matrix Estimation: Existence and High Dimensional Consistency
Source: arXiv:2111.00590 source file (2022-02-23)
Supplement: Supplementary file 1 [file appendix.tex]

\subsection{Strict convexity of Stein loss}
\label{ap_strict_convexity_loss}
The Hessian is an $\vert \Ec \vert \times \vert \Ec \vert$ real matrix. For a pair of edges $e=(i,j)$ and $f=(s,t)$ in   $\Ec$,   the   $(e,f)$ entry of $\Zm$ is given by
 \begin{align}
     z_{ef} =  - \frac{\partial r_e}{\partial w_f} = \left( \frac{-r_{is} + r_{it} + r_{js} - r_{jt}}{2}  \right)^2.
 \end{align}
 Let  $\xv \neq \mathbf{0}$, then 
\begin{equation*}
    \xv^{\top}\Zm \xv = \sum_{e \in \Ec} \sum_{f \in \Ec} x_e x_f z_{ef} \geq  \sum_{e \in \Ec} x^2_e z_{ee} = \sum_{e \in \Ec} x^2_e r^2_{e} >0.
\end{equation*}
The last equality is strict because for connected graphs, $r_{e}>0$ for all $e \in [p]^2$.
